# Supplementary material for: Paper2SysArch: Structure-Constrained System Architecture Generation from Scientific Papers
Source: arXiv:2511.18036 ancillary file (2025-11-22)
Supplement: Supplementary file 1 [file Browsing_Like_Human_-_A_Multimodal_Web_Agent_with_Experiential_Fast-and-Slow_Thinking.pdf]

# Browsing Like Human: A Multimodal Web Agent with Experiential Fast-and-Slow Thinking

Haohao Luo<sup>1\*</sup>, Jiayi Kuang<sup>1</sup>, Wei Liu<sup>2</sup>, Ying Shen<sup>1,4†</sup>, Jian Luan<sup>2</sup>, Yang Deng<sup>3</sup>

<sup>1</sup>Sun Yat-sen University    <sup>2</sup>MiLM Plus, Xiaomi Inc    <sup>3</sup>Singapore Management University  
<sup>4</sup>Guangdong Provincial Key Laboratory of Fire Science and Intelligent Emergency Technology  
{luohh5,kuangjy6}@mail2.sysu.edu.cn    {liuwei40,luanjian}@xiaomi.com  
sheny76@mail.sysu.edu.cn    ydeng@smu.edu.sg

## Abstract

Automating web navigation which aims to build a web agent that follows user instructions to complete tasks like booking flights by interacting with websites, has received increasing attention due to its practical value. Although existing web agents are mostly equipped with visual perception, planning, and memory abilities, their reasoning process are still deviate from human cognition. In this work, we study the human thought pattern to empower agent with more human-like abilities in web navigation. To tackle this problem, we propose a novel multimodal web agent framework called WebExperT, which is designed to emulate the human planning process of "thinking fast and slow" to effectively decompose complex user instructions. Furthermore, WebExperT leverages experiential learning by reflecting from failure for continuously refining planning and decision-making outcomes. Experimental results on the MIND2WEB benchmark demonstrate the superiority of WebExperT in both supervised and unsupervised settings.

## 1 Introduction

Automating web navigation (Deng et al., 2023; He et al., 2024) refers to a category of sequential decision-making problems where agents follow user instructions to complete tasks on any given website by controlling browsers. Common web navigation tasks include booking tickets via a sequence of interactions with computer interface such as *Click* or *Type*. As shown in Figure 1, a key aspect of automating web navigation is observing and perceiving from the website environment through leveraging inputs like HTML text and rendered screenshots. With the advent of multimodal LLMs, the perception paradigms in recent web agents have shifted from text-based (Yao et al., 2022; Ma et al.,

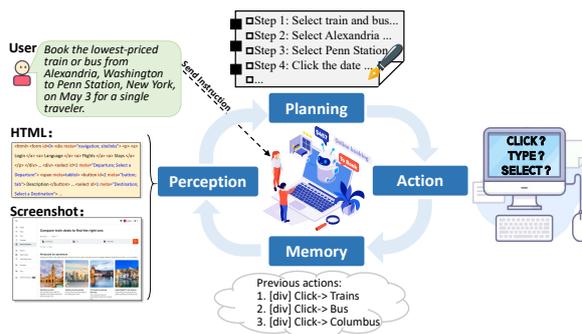

Figure 1: Overview of the web navigation problem.

2023) paradigm to multimodal (Zhou et al., 2024; Lee et al., 2023) paradigm. Despite these advances, existing web agents still struggle in browsing as effectively as humans, since their reasoning patterns differ from human cognition a lot.

To make the web agent behave more like a human, recent studies focus on empowering web agents with planning (Zheng et al., 2024c; Gur et al., 2024; Kim et al., 2023a) and memory (Wang et al., 2024c; Deng et al., 2024b) abilities. As illustrated in Figure 1, when faced with complex user instructions, multimodal web agent with planning ability can break down the instructions into a sequence of necessary steps or sub-tasks, while the memory mechanism helps revisit and apply antecedent strategies effectively. However, the planning mechanisms in existing multimodal web agents, which typically rely on zero-shot prompting or in-context learning of multimodal LLMs, are often limited to single-step reasoning that deviates significantly from human cognitive processes. Moreover, human learning often occurs by extracting insights from experiences, enabling generalization to novel situations, but most web agents proposed in current studies are limited to short-term memory (previous trajectories) rather than long-term memory (experiences). Such difference of thought patterns results in their inferior performance to humans in web navigation.

In this work, we propose WebExperT, a multi-

\* Work was done during a remote internship at SMU.

† Corresponding author.

modal web agent that emulates the human thought pattern of "thinking fast and slow" (Kahneman, 2011). Dual-process theory posits that human cognition is composed of two distinct manners: (1) **Slow and analytic** thinking for deliberate reasoning, (2) **Fast and heuristic** thinking for intuitive judgments. This dual-process mechanism is a fundamental aspect of human skill acquisition. At the initial stages of learning, due to lack of experience, humans rely on slow and deliberate thinking to reason step by step and consolidate knowledge through trial-and-error and reflection analysis. Over time, this knowledge becomes internalized, forming "muscle memory" that supports fast and instinctive reactions in familiar scenarios. Specifically, WebExperT first marks interactive web elements on screenshots with bounding boxes and employs multimodal LLMs for encoding. Then we introduce a dual-process planning mechanism, where slow thinking is employed for deliberately generating comprehensive plans step-by-step and transferring knowledge to the lightweight model in fast thinking through supervised fine-tuning. When failure occurs, the experience will be stored in memory and employed to generate natural language insights through self-reflection, helping the agent learn from prior mistakes as experiential learning.

Our contributions are summarized as follows:

- We propose a novel multimodal web agent framework, called WebExperT, designed to emulate the human planning process. The framework incorporates a dual-process planning mechanism, enabling fast thinking to leverage the capabilities of slow thinking for effectively decomposing complex multimodal tasks.
- WebExperT further enhances its planning capabilities by consolidating experiential knowledge through trial-and-error processes and reflective analysis, enabling continuous refinement of its planning outcomes.
- Experimental results on the MIND2WEB benchmark show that WebExperT outperforms existing methods and effectively takes advantage of fast-and-slow thinking. Our code will be released via <https://github.com/Luohh5/WebExperT>.

## 2 Related Works

**Web Agent** Evolving from early simulated web environment data (Liu et al., 2018; Mazumder and Riva, 2021; Wang et al., 2024b), many high-quality real-world data have been proposed to explore web navigation challenges in more realistic and com-

plex scenarios, with focusing on a wide range of web domains and task types (Deng et al., 2023), realistic and reproducible web environments (Zhou et al., 2024), and visual UI understanding (Zheng et al., 2024a). Based on these data, many studies develop agents with LLM large-scale finetuning (Gur et al., 2024), prompting LLM (Kim et al., 2023b), and reinforcement learning (Humphreys et al., 2022). Recent studies extend multimodal web agents by solely relying on screenshots input (Shaw et al., 2023), integrating screenshots with HTML data to enhance website comprehension (Furuta et al., 2024), and marking interactive web elements on screenshots (He et al., 2024).

**Planning Mechanisms of Agents** Planning plays a crucial role in solving complicated problems in daily human life (Deng et al., 2024a; Zhang et al., 2024), and it is also a fundamental capability for agents. Evolving from prior research (Shen et al., 2023; Yao et al., 2023b) based on divide-and-conquer approaches, most existing studies decompose complex tasks by Monte Carlo Tree Search (Zhao et al., 2023), A\* (Xiao and Wang, 2023), or Breadth-First Search (Yao et al., 2023a). Another line of studies (Guan et al., 2023; Dagan et al., 2023) combines symbolic planners with LLM agents to create natural language plans. With the development of LLMs, recent works (Kim et al., 2023b; Xie and Zou, 2024) design various finetuning and prompting strategies to enhance the planning abilities of agents. To make planning more akin to humans, our work enhance the agent’s planning mechanism with the human thought pattern of "fast and slow thinking".

**Memory Mechanisms of Agents** Just as humans leverage prior thoughts, actions, and observations for decision-making, agents require memory mechanisms to handle complex tasks effectively. Inspired by the progression of human memory from short-term to long-term, early approaches use in-context learning to build short-term memory systems for various applications (Fischer, 2023; Song et al., 2023; Wang et al., 2024a). To consolidate important information over time, recent studies (Park et al., 2023; Zhu et al., 2023; Lin et al., 2023) leverage long-term memory pool to store prior experiences, which can not only serve as exemplars (Zheng et al., 2024c; Luo et al., 2024) to guide actions but also allow agents to learn from error-and-trial (Shinn et al., 2023; Zhao et al., 2024a). In this work, we combine the experiential learning

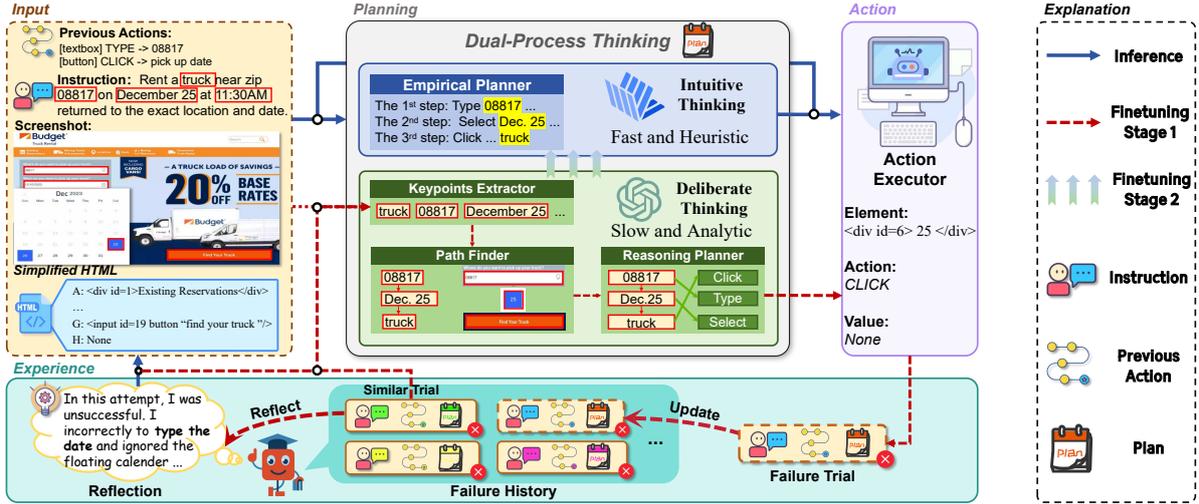

Figure 2: The overall framework of WebExpertT. For instance, the user instruction, “Rent a truck ... and date.” contains critical constraints such as the vehicle type “truck,” zip code “08817,” date “December 25,” and time “11:30 AM.” The dual-process planning breaks down the instruction into subtasks, e.g., “Step 1: Type 08817 ... Step 2: Select Dec. 25 ... Step 3: Click ... truck ...,” providing structured guidance for action generation. When encountering errors, reflective feedback like “... incorrectly to type the date ...” helps the agent learn from past failures.

and planning mechanism to empower web agents with more human-like reasoning abilities.

### 3 WebExpertT

Given a real-world website  $\mathcal{W}$  and user instruction  $q$ , multimodal web agent aims to generate the executable action sequence  $\mathcal{A} = [a_1, a_2, \dots, a_n]$ , where action  $a_t$  at time step  $t$  is determined based on  $q$ , observation of the current webpage environment  $w_t$ , and previous actions sequence  $\mathcal{A}_{t-1} = [a_1, a_2, \dots, a_{t-1}]$ . Specifically, the environment observation  $w = \{s, h\}$  consists of a screenshot  $s$  and HTML texts  $h$  of the website. Each action  $a = \{e, o, v\}$  represents a triplet comprising three essential variables for a browser event, where  $e \in \mathcal{E}$  identifies the interactive element (e.g., search bar) selected from the interactive elements set  $\mathcal{E}$  in website, and  $o$  specifies the corresponding operation (e.g., *Click* or *Type*) chosen from the set of predefined operations  $\mathcal{O}$ . The variable  $v$  provides any additional value required for the corresponding operation (e.g., zip code 08817 for a *Type* operation).

#### 3.1 Architecture

As illustrated in Figure 2, we first process the environment observation by simplifying HTML content and grounding the interactive elements in rendered screenshot. Following the MINDACT framework (Deng et al., 2023), we employ a small pre-trained language model (e.g., DeBERTa (He et al., 2021)) to rank the top- $N$  candidates DOM ele-

ments  $\mathcal{C} = \{c_1, c_2, \dots, c_N\}$  that are most relevant to the task and the current status. Then we follow (Zheng et al., 2024b) to overlay a bounding box with a label for each candidate element on screenshot  $s^{box}$ . To generate high-quality plans, we introduce a dual-process planning mechanism  $\mathcal{F}_{plan} = \{\mathcal{F}_{fast}, \mathcal{F}_{slow}\}$  with reference to the human thought pattern of “thinking fast and slow”. Supervised by groundtruth action  $\hat{a}_t$ , we finetune the action executor  $\mathcal{F}_{action}$  to leverage the generated plan as guidance to execute action  $a_t$ . To induce longer-horizon planning and better action through feedback, we introduce an experiential learning mechanism to generate insights from failure history via self-reflection  $\mathcal{F}_{reflect}$ .

#### 3.2 Dual-Process Planning

To empower multimodal web agent with more human-like planning abilities, we introduce a dual-process planning mechanism that emulates the human thought pattern of “thinking fast and slow” (Kahneman, 2011), featuring deliberate thinking process and intuitive thinking process.

**Deliberate Thinking Process** User instructions may involve numerous constrained requirements (e.g., price), making it challenging for agent to understand. Therefore, we design a deliberate thinking process to decompose the instructions into subtasks based on the key requirements. Specifically, we first introduce a keypoints extractor module  $\mathcal{G}_{KE}$  to identify the key requirements in the in-

struction as keypoints  $\mathcal{K} = \{k_1, k_2, \dots, k_m\}$  that need to be considered by the action executor:

$$\mathcal{K} = \mathcal{G}_{KE}(q, s), \quad (1)$$

Subsequently, to mimic the human web browsing habits and the logic of web design (from top to bottom, from left to right), we propose a path finder module  $\mathcal{G}_{PF}$  to generate a rough route  $\mathcal{K}_r$  based on the identified keypoints and their position in screenshot:

$$\mathcal{K}_r = \mathcal{G}_{PF}(\mathcal{K}, s), \quad (2)$$

Finally, we develop a reasoning planner module  $\mathcal{G}_{RP}$  to complement the corresponding operation and other information of each keypoint in generated route as golden plan  $\hat{p}$ :

$$\hat{p} = \mathcal{F}_{slow}(q, s) = \mathcal{G}_{RP}(\mathcal{K}_r, s), \quad (3)$$

By employing these three modules, we introduce a Chain-of-Thought reasoning strategy (Wei et al., 2022) to make planning step-by-step. Note that the deliberate thinking process is only triggered in training procedure and implemented with off-the-shelf multimodal language models (details in Appendix A), leveraging their world knowledge to drive the three modules.

**Intuitive Thinking Process** While the deliberate thinking process can make more comprehensive planning due to its careful consideration, the slowness of multi-step reasoning results in higher web interaction latency, limiting its practical usability in real-world scenarios. In fact, humans often utilize an empirical thinking pattern by forming muscle memory through repeated practice. Inspired by this, we design an intuitive thinking process to perform single-step inference by incorporating a lightweight model to inherit the planning ability of deliberate thinking. Specifically, we perform supervised fine-tuning using the golden plans  $\hat{p}$  in deliberate thinking process to distill knowledge into the lightweight language model:

$$p = \mathcal{F}_{fast}(q, s) = \mathcal{G}_{EP}(q, s), \quad (4)$$

where  $p$  denotes the plan generated by empirical planner  $\mathcal{G}_{EP}$  in intuitive thinking process. By this means, the intuitive thinking process exhibits capabilities comparable to deliberate thinking and improves the planning efficiency.

---

### Algorithm 1 Two-Stage Training Procedure

---

**Require:** The action executor  $\mathcal{F}_{action}$  and its parameters  $\theta_a$ , the empirical planner  $\mathcal{F}_{fast}$  and its parameters  $\theta_s$ , the failure history pool  $\mathcal{M}$ , the training dataset  $\mathcal{D}$ .

- 1: Initialize the failure history pool  $\mathcal{M} = \emptyset$
- 2: // Stage 1: Finetuning Action Executor
- 3: **for**  $\{\mathcal{A}_{t-1}, q, s^{box}, \mathcal{C}, \hat{a}_t\} \in \mathcal{D}$  **do**
- 4:    $\hat{p} \leftarrow \mathcal{F}_{slow}(q, s)$
- 5:   Generate  $a_t = \mathcal{F}_{action}(\mathcal{A}_{t-1}, q, s^{box}, \mathcal{C}, \hat{p})$  supervised by  $\hat{a}_t$
- 6:   Update  $\theta_a$  by optimizing  $\mathcal{L}(a_t, \hat{a}_t)$  via Eq. (7)
- 7:   **if**  $a_t \neq \hat{a}_t$  **then**
- 8:     Update  $\mathcal{M}$  by adding the failure trial  $m = (\mathcal{A}_{t-1}, q, \hat{p})$
- 9:   **end if**
- 10: **end for**
- 11: // Stage 2: Finetuning Empirical Planner
- 12: **for**  $\{\mathcal{A}_{t-1}, q, s^{box}, \mathcal{C}, \hat{a}_t\} \in \mathcal{D}$  **do**
- 13:   **if**  $\mathcal{M} \neq \emptyset$  **then**
- 14:     Retrieve top- $k$  relevant trials  $\{m_1, m_2, \dots, m_k\}$  from history failure pool  $\mathcal{M}$  via Eq. (9)
- 15:      $r \leftarrow \mathcal{F}_{reflect}(m_1, m_2, \dots, m_k)$
- 16:     Refine the golden plan  $\hat{p}_r \leftarrow \mathcal{F}_{slow}(q, s, r)$
- 17:     Generate  $p = \mathcal{F}_{fast}(q, s)$  supervised by  $\hat{p}_r$
- 18:     Update  $\theta_s$  by optimizing  $\mathcal{L}(p, \hat{p}_r)$  via Eq. (7)
- 19:   **end if**
- 20: **end for**

---

### 3.3 Experiential Learning

Inspired by the cognitive abilities inherent in human learning, we develop an experiential learning mechanism to improve our agent’s decision-making and planning capabilities through error-and-trial. Specifically in training procedure, we construct a failure history pool  $\mathcal{M}$  to store the failure trials. For each failure trial  $m = \{\mathcal{A}_{t-1}, q, \hat{p}\}$ , we keep the user instruction, previous actions, and golden plan in mind while discarding the rest. Then the agent retrieves from  $\mathcal{M}$  with top- $k$  task-relevant trials  $\{m_1, m_2, \dots, m_k\}$  (details in Appendix A) and extracts insights as reflection  $r$  from them to learn from experiences of a behavior policy:

$$r = \mathcal{F}_{reflect}(m_1, m_2, \dots, m_k), \quad (5)$$

A part of reflections related to planning are treated as verbal feedback (Shinn et al., 2023) to refine the deliberate thinking process, and other reflections are added into the prompt of action executor to guide decision-making for future trial by

$$a_t = \mathcal{F}_{action}(\mathcal{A}_{t-1}, q, s^{box}, \mathcal{C}, p, r), \quad (6)$$

Experiential learning helps our agent identify the reasons for failure and avoid repeating mistakes in decision-making and planning phase.

### 3.4 Two-Stage Training Procedure

We design a two-stage training procedure to train WebExperT by supervised finetuning multimodal

---

**Algorithm 2** Inference Procedure

---

**Require:** The action executor  $\mathcal{F}_{action}$ , the empirical planner  $\mathcal{F}_{fast}$ , the reflection generator  $\mathcal{F}_{reflect}$ , the failure history pool  $\mathcal{M}$  from training procedure, the test dataset  $\mathcal{D}_t$ .

- 1: **for**  $\{\mathcal{A}_{t-1}, q, s^{box}, C\} \in \mathcal{D}_t$  **do**
  - 2:    $p \leftarrow \mathcal{F}_{fast}(q, s)$
  - 3:   Retrieve top-k relevant trials  $\{m_1, m_2, \dots, m_k\}$  from history failure pool  $\mathcal{M}$  via Eq. (9)
  - 4:    $r \leftarrow \mathcal{F}_{reflect}(m_1, m_2, \dots, m_k)$
  - 5:   Generate  $a_t = \mathcal{F}_{action}(\mathcal{A}_{t-1}, q, s^{box}, p, r)$
  - 6: **end for**
- 

LLMs, as shown in Algorithm 1.

**Stage 1: Finetuning Action Executor** We employ the user input  $U_t = \{\mathcal{A}_{t-1}, q, s^{box}, C\}$  and golden plan  $\hat{p}$  to finetune action executor  $\mathcal{F}_{action}$ .

**Stage 2: Finetuning Empirical Planner** The reflections about planning generated from the failure trials in Stage 1 will refine the golden plan  $\hat{p}$ , which will subsequently be utilized to finetune the empirical planner  $\mathcal{F}_{fast}$  for intuitive thinking.

In each stage, we have the same training objective that minimizes the sum of negative log-likelihood loss averaged over tokens:

$$\mathcal{L}(y, \hat{y}) = -\frac{1}{L} \sum_{l=1}^L \hat{y}_l \log \left( \frac{\exp(y_l)}{\sum_i \exp(y_i)} \right), \quad (7)$$

where  $L$  is the max length of output sequence,  $\hat{y}_l$  and  $y_l$  denote the  $l$ -th token in the groundtruth sequence  $\hat{y}$  and generation sequence  $y$ , respectively.

**Inference Procedure** Given the user input  $I_t$ , empirical plan  $p$ , and reflections  $r$  from experience, the action executor attempts unseen tasks with action  $a_t$  as Eq. (6) during inference, as shown in Algorithm 2. Note that the failure history pool only gathers experience from training procedure and will not be updated during inference to further reduce the latency in real-world application.

## 4 Experiment

### 4.1 Experimental Setups

**Datasets** We evaluate on MIND2WEB (Deng et al., 2023), a comprehensive dataset designed for real-world web navigation, featuring over 2,000 complex web tasks collected from 137 real-world websites spanning 31 different domains, such as travel and shopping. It supports key operations like Click, Type, and Select, with Hover and Press Enter incorporated into Click to minimize ambiguity. The test splits are designed to evaluate web agents’ generalization across tasks, websites, and

---

| Split         | # Tasks | # Domains | # Websites | Avg # Actions |
|---------------|---------|-----------|------------|---------------|
| Train         | 1,009   | 17        | 73         | 7.7           |
| Cross-Task    | 177     | 17        | 64         | 7.6           |
| Cross-Website | 142     | 9         | 10         | 7.2           |
| Cross-Domain  | 694     | 13        | 53         | 5.9           |

---

Table 1: Dataset statistics of MIND2WEB.

domains. **Cross-Task** setting tests agents on unseen tasks within included domains and websites. **Cross-Website** setting introduces tasks from 10 new websites per top-level domain. **Cross-Domain** setting assesses performance on tasks from two entirely unseen top-level domains. The details of dataset statistics are presented in Table 1.

**Evaluation Metrics** We adopt four metrics that are widely used for web agent evaluation: 1) **Time Cost** calculates the average inference time in second. 2) **Element Accuracy** (Ele. Acc) compares the selected element with the ground-truth elements. 3) **Operation F1** (Op. F1) calculates the token-level F1 score for the predicted operation and additional value. 4) **Step Success Rate** (Step SR) measures the success of each step; A step is considered successful only if both the selected element and the predicted operation are correct. For each step, they provide previous “groundtruth” actions with the assumption that the model successfully completes all previous steps.

**Baselines** Besides the general baseline in MIND2WEB, *i.e.*, MINDACT (Deng et al., 2023), we compare WebExperT with the state-of-the-art multimodal web agent frameworks, including SEEACT (Zheng et al., 2024b), Auto-Intent (Kim et al., 2024), WebGUM (Furuta et al., 2024) for supervised finetuning (SFT) and GPT (OpenAI, 2023), CogAgent (Hong et al., 2024) for in-context learning (ICL). Notably, we employ the same multimodal LLM, Flan-T5 (Chung et al., 2024), as the backbones of all baselines for SFT to prevent the impact caused by the differences of different models’ power. More details about baselines and experimental setups are presented in Appendix A.

### 4.2 Overall Performance

**Offline Evaluation Results** Table 2 compares WebExperT with previous state-of-the-art models, showing its consistent outperformance across three test splits. Moreover, WebExperT’s performance improves with larger backbone models, highlighting its adaptability to advanced multimodal LLMs.

Regarding the ICL setting, GPT-4o, with its multimodal reasoning abilities and knowledge, outper-

| Method                          | Base Model               | Time Cost   | Cross-Task  |             |             | Cross-Website |             |             | Cross-Domain |             |             |
|---------------------------------|--------------------------|-------------|-------------|-------------|-------------|---------------|-------------|-------------|--------------|-------------|-------------|
|                                 |                          |             | Ele.Acc     | Op. F1      | Step SR     | Ele.Acc       | Op. F1      | Step SR     | Ele.Acc      | Op. F1      | Step SR     |
| <b>In-Context Learning</b>      |                          |             |             |             |             |               |             |             |              |             |             |
| Few-shot                        | GPT-3.5                  | <b>0.9s</b> | 19.4        | 59.2        | 16.8        | 14.9          | 56.5        | 14.1        | 25.2         | 57.9        | 24.1        |
| Few-shot                        | GPT-4                    | <u>1.3s</u> | 40.8        | 63.1        | 32.3        | 30.2          | 61.0        | 27.0        | 35.4         | 61.9        | 29.7        |
| Few-shot                        | GPT-4o                   | 3.5s        | 42.0        | 63.9        | 32.8        | 31.5          | 61.3        | 27.9        | 36.6         | 62.1        | 30.5        |
| CogAgent (Hong et al., 2024)    | CogAgent <sub>18B</sub>  | 4.7s        | 22.4        | 53.0        | 17.6        | 18.4          | 42.2        | 13.4        | 20.6         | 42.0        | 15.5        |
| WebExperT                       | GPT-4o                   | 16.2s       | 45.6        | 67.4        | 39.2        | 39.3          | 63.5        | 36.4        | 42.9         | 64.9        | 37.1        |
| <b>Supervised Fine-Tuning</b>   |                          |             |             |             |             |               |             |             |              |             |             |
| MINDACT (Deng et al., 2023)     | Flan-T5 <sub>XL</sub>    | 9.5s        | 55.1        | 75.7        | 52.0        | 42.0          | 65.2        | 38.9        | 42.1         | 66.5        | 39.6        |
| SEEACTION (Zheng et al., 2024b) | Flan-T5 <sub>XL</sub>    | 10.7s       | 52.9        | 74.9        | 50.3        | 41.7          | 74.1        | 38.3        | 43.8         | 73.4        | 39.6        |
| Auto-Intent (Kim et al., 2024)  | Flan-T5 <sub>XL</sub>    | -           | 55.8        | 73.3        | 50.1        | 47.6          | 64.0        | 40.0        | <u>47.3</u>  | 66.3        | 42.5        |
| WebGUM (Furuta et al., 2024)    | Flan-T5 <sub>XL</sub>    | -           | <u>57.2</u> | 80.3        | <u>53.7</u> | 45.3          | 70.9        | 41.6        | 43.9         | 72.2        | 41.4        |
| WebExperT                       | Flan-T5 <sub>Base</sub>  | 14.9s       | 45.2        | 81.5        | 41.1        | 44.9          | 77.0        | 39.4        | 38.3         | 78.1        | 33.9        |
| WebExperT                       | Flan-T5 <sub>Large</sub> | 15.1s       | 55.0        | <u>83.1</u> | 49.9        | <u>49.1</u>   | <u>78.2</u> | <u>43.7</u> | 44.8         | <u>81.0</u> | 40.4        |
| WebExperT                       | Flan-T5 <sub>XL</sub>    | 15.4s       | <b>60.3</b> | <b>84.4</b> | <b>54.9</b> | <b>53.9</b>   | <b>79.6</b> | <b>49.0</b> | <b>48.5</b>  | <b>81.5</b> | <b>44.0</b> |

Table 2: Offline evaluation results on MIND2WEB dataset.

| Method                      | Cross-Task  |             |             | Cross-Website |             |             | Cross-Domain |             |             |
|-----------------------------|-------------|-------------|-------------|---------------|-------------|-------------|--------------|-------------|-------------|
|                             | Ele.Acc     | Op. F1      | Step SR     | Ele.Acc       | Op. F1      | Step SR     | Ele.Acc      | Op. F1      | Step SR     |
| WebExperT                   | <b>60.3</b> | <b>84.4</b> | <b>54.9</b> | <b>53.9</b>   | <b>79.6</b> | <b>49.0</b> | <b>48.5</b>  | <b>81.5</b> | <b>44.0</b> |
| - w/o Intuitive Thinking    | 60.1        | 84.4        | 54.8        | 53.8          | 79.6        | 48.9        | 48.3         | 81.4        | 43.9        |
| - w/o Deliberate Thinking   | 57.6        | 82.6        | 53.7        | 47.0          | 77.1        | 43.0        | 45.3         | 80.2        | 42.5        |
| - w/o Dual-Process Planning | 56.1        | 82.4        | 53.6        | 46.5          | 76.1        | 42.2        | 44.9         | 79.8        | 42.5        |
| - w/o Experiential Learning | 59.3        | 84.1        | 54.2        | <u>52.7</u>   | 77.9        | 48.1        | 47.3         | 80.4        | 43.2        |
| - w/o Screenshot            | 58.4        | 83.2        | 52.6        | 52.5          | 79.4        | 46.7        | 47.9         | 79.5        | 43.2        |
| - w/o HTML                  | 34.0        | 82.3        | 29.6        | 33.9          | 78.4        | 29.7        | 29.0         | 79.8        | 25.1        |

Table 3: Ablation study of WebExperT with Flan-T5<sub>XL</sub>.

forms GPT-3.5, GPT-4 and CogAgent among ICL baselines but fails to surpass WebExperT. Leveraging its well-designed planning and experiential learning, WebExperT outperforms GPT-4o by 6.4%, 8.5%, and 6.6% Step SR in Cross-Task, Cross-Website, and Cross-Domain settings, respectively.

Regarding the SFT setting, all ICL methods significantly lag behind SFT methods, underscoring SFT’s superiority in web agents. Specifically, despite leveraging visual input, SEEACTION offers no advantage over MINDACT due to CLIP’s limited ability to capture image details essential for web navigation (Shen et al., 2022). Furthermore, Auto-Intent which extends web agent with intent discover ability outperforms SEEACTION and MINDACT in Cross-Website and Cross-Domain splits. Although WebGUM demonstrates better perception and multi-step reasoning, it falls short of WebExperT. WebExperT achieves a 1.2% Step SR improvement in Cross-Task settings and leads by 7.4% and 4.4% in Cross-Website and Cross-Domain settings, respectively. The consistent high performance across ICL and SFT further validates WebExperT’s effectiveness.

Additionally, across the three test splits, most methods in both ICL and SFT perform better on tasks seen during training, except GPT-3.5. However, compared to strongest baseline such as WebGUM and Auto-Intent, the relative improvement of WebExperT on Cross-Domain split is higher than that on Cross-Task split. Therefore, the consistent performance across tasks, websites, and domains, highlighting the generalizability and scalability of our WebExperT framework.

However, well-crafted web agent framework such as SEEACTION and MINDACT generally incur higher time costs compared to the few-shot methods. This is because the effective sub-modules (e.g. element grounding) enhance decision-making performance but also increase computational overhead. Similarly, while the dual-process planning and experiential learning mechanisms in WebExperT do result in higher time costs than GPT-4o by 11.9s, they also enable the system to achieve the best decision-making performance. Meanwhile, a latency of approximately 15 seconds is acceptable in the context of existing automated web navigation studies and exhibits promising practical usability. More details about the time cost of dual-process

| Method     | Whole Task SR(%) |
|------------|------------------|
| FLAN-T5-XL | 8.9              |
| GPT-4      | 13.3             |
| SEEACT     | 31.5             |
| WebExperT  | <b>33.2</b>      |

Table 4: Online evaluation results of MIND2WEB tasks.

planning are presented in Section 4.4.

**Online Evaluation Results** Following the settings of SEEACT (Zheng et al., 2024b), we pair a web agent with a human annotator to conduct online evaluation experiments of MIND2WEB tasks in real-world browser, where the human annotator’s task was to monitor agent’s actions that may alter real-world states and determine whether each task was completed successfully. And we utilize the Whole Task Success Rate as the evaluation metric. Additionally, we re-write time-sensitive tasks to ensure they are still valid when the evaluation is conducted. For instance, we update the dates for flight-related tasks. Furthermore, the online evaluation was conducted on a subset of 90 tasks from the three test splits. As shown in Table 4, SEEACT with well-designed web agent framework outperforms both GPT-4 and FLAN-T5-XL by a large margin of over 20% whole task success rate. Additionally, despite leveraging GPT-4’s superior generalization capabilities, SEEACT still fails to outperform the fine-tuned WebExperT in terms of the Whole Task Success Rate. This demonstrates that fine-tuned frameworks do not necessarily have poor real-world applicability, as long as they are equipped with sufficiently well-crafted scalability enhancement modules. These results further confirm the potential of our WebExperT framework for real-world scenario usability.

### 4.3 Ablation Study

As summarized in Table 3, we conduct ablation studies of WebExperT in SFT setting to assess the impact of each component and leave additional results of ICL setting in Appendix B. There are several notable observations as follows:

- In dual-process planning, "w/o Intuitive Thinking" refers to using deliberate thinking in place of intuitive thinking during inference stage, which measures the extent to which intuitive thinking inherits the capabilities of deliberate thinking. The minor performance decline demonstrates a better inheritance and successfully developing "muscle

| Modules      | Rel.        | Coh.        | Mat.        | Overall     |
|--------------|-------------|-------------|-------------|-------------|
| RP           | 3.82        | 3.91        | 4.07        | 3.94        |
| KE + RP      | 4.64        | 4.02        | 4.18        | 4.19        |
| PF + RP      | 4.01        | 4.19        | 4.03        | 4.13        |
| KE + PF + RP | <b>4.64</b> | <b>4.23</b> | <b>4.31</b> | <b>4.59</b> |

Table 5: Human evaluation of golden planner generation with difference module collocations. KE: Keypoint Extractor, PF: Path Finder, RP: Reasoning Planner

| Base Model               | Cross-Task  |             | Cross-Website |             | Cross-Domain |             |
|--------------------------|-------------|-------------|---------------|-------------|--------------|-------------|
|                          | B-4         | R-L         | B-4           | R-L         | B-4          | R-L         |
| <b>Empirical Planner</b> |             |             |               |             |              |             |
| - InternVL2              | <b>75.8</b> | <b>74.2</b> | <b>83.2</b>   | <b>83.6</b> | <b>80.1</b>  | <b>79.8</b> |
| - Qwen-VL                | 74.9        | 74.2        | 75.2          | 73.5        | 78.3         | 75.0        |
| - LLaVA                  | 74.8        | 73.9        | 78.5          | 78.1        | 76.3         | 74.5        |
| - InstructBLIP           | 71.2        | 70.5        | 69.1          | 69.7        | 68.8         | 67.7        |

Table 6: Detailed performance of empirical planner with different base models.

memory" through training. Additionally, "w/o Deliberate Thinking", which means discarding the deliberate thinking in training stage, causes Step SR to drop by 1.2%, 6.0%, and 1.5% in Cross-Task, Cross-Website, and Cross-Domain splits, respectively. Moreover, eliminating the entire planning module leads to most sharp declines across all splits, with a notable 6.8% drop in Cross-Website performance, further validating the effectiveness of "fast and slow thinking" in planning.

- When we drop experiential learning mechanism, We can see a performance decrease of 0.7%, 0.9%, and 0.8% Step SR across three test splits, which demonstrates that the experience and reflection extracted from failure history indeed help WebExperT avoid repeated mistakes and refine its decision-making.
- As for the environment observation, dropping either the rendered screenshot or the HTML document results in a substantial decline in performance across three test splits, particularly with a 2.3% and 25.3% decrease in Cross-Task split. It highlights the advantages of incorporating both visual and textual information in automating web navigation task.

### 4.4 Further Analysis

**Analysis of Deliberate Thinking** To further investigate whether the golden plans are appropriate enough to supervise the finetuning of empirical planner, we conduct a human evaluation to evaluate the quality of golden plans generated in deliberate

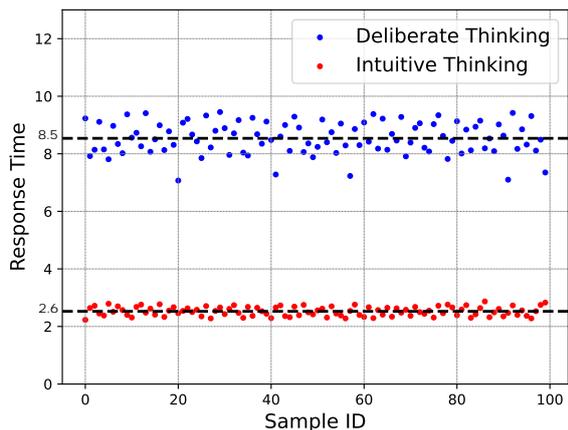

Figure 3: The response time of fast-and-slow thinking.

thinking process. Specifically, we randomly select 50 golden plan samples and employ three annotators in our lab to rate them from 1 (worst) to 5 (best) based on 4 metrics: (1) **Relevance (Rel.)**: measures whether the golden plans capture all the key requirements in user instruction; (2) **Coherence (Coh.)**: measures whether the orders of golden plans are aligned with human web browsing habit; (3) **Match (Mat.)**: measures whether the operations in golden plans match the corresponding element in screenshot; (4) **Overall**: measures whether the plan is effective enough to guide decision-making. All annotators are graduate student major in computer science with native-level fluency in English. Clear and detailed guideline is provided to the annotators to ensure consistency and reliability in their evaluations, as presented in Appendix E.

Table 5 presents human evaluation results for golden planner generation with different module configurations. Our deliberate thinking process, utilizing all three modules, achieves an impressive **Overall** score of 4.59, validating the quality of the generated plans. Removing any module results in performance declines across all metrics, while relying solely on the reasoning planner for single-step reasoning yields the poorest performance among all configurations.

**Analysis of Intuitive Thinking** To assess knowledge transfer from the reasoning planner to the empirical planner, we use BLEU-4 (Papineni et al., 2002) and ROUGE-L (Lin, 2004) to evaluate the match between the empirical plan  $p$  and the golden plan  $\hat{p}$ . As shown in Table 6, the empirical planner achieves 83.2 BLEU-4 and 83.6 ROUGE-L in the Cross-Website split, demonstrating it effectively inherits the reasoning planner’s capabilities

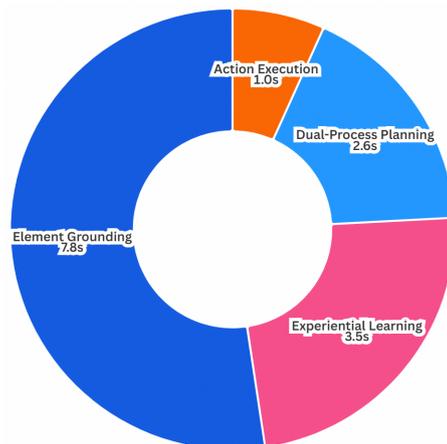

Figure 4: The response time of all modules in WebExpert.

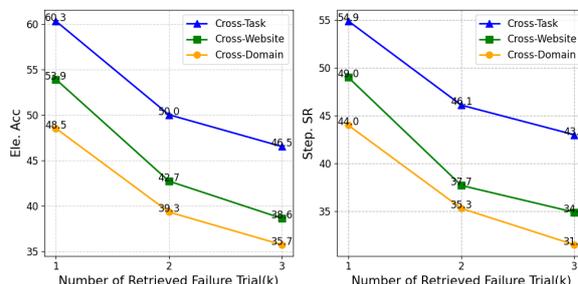

Figure 5: The overall performance with varying number of retrieved failure trials.

and forms "muscle memory" through practice. To validate InternVL2 (Chen et al., 2024) as the base model for the empirical planner, we compare it against Qwen-VL (Bai et al., 2023), LLaVA (Liu et al., 2023), and InstructBLIP (Dai et al., 2023), using identical prompts for fairness. Table 6 shows InternVL2 outperforms the alternatives, highlighting its suitability for the empirical planner. Despite minor performance differences among the base models, all show strong results across test splits, confirming the effectiveness and versatility of our dual-process planning framework.

**Analysis of Time Cost** In real-world scenarios, time cost is a critical metric for evaluating the usability of an agent. However, as mentioned in Section 4.2, well-crafted frameworks with more components tend to incur higher time costs. To address this challenge, we propose intuitive thinking process to speed up planning by employing single-step reasoning. To justify the effectiveness and superiority of intuitive thinking in efficiency, we conduct an experiment to evaluate and compare the time costs of intuitive thinking and deliberate thinking. Specifically, we create a subset of total 100 samples by randomly selecting instances from

the three test splits and measure the response times for dual-process thinking when making planning on this subset. As shown in Figure 3, deliberate thinking generally requires 7.5 to 10 seconds to perform multi-step planning, with an average response time of 8.5 seconds. In contrast, the response times of intuitive thinking remain consistently below 3 seconds and have an average response time of 2.6 seconds, which is over 3 times faster than deliberate thinking. Therefore, intuitive thinking can indeed be witnessed to speed up the planning process and improve inference efficiency. Furthermore, we utilize the same setting to evaluate the response latency of each component in WebExperT to further investigate the time cost distribution of our framework. As shown in Figure 4, the Element Grounding module incurs the highest time cost during inference, which we follow MINDACT and SEEACT to design it. Therefore, it's obvious to find that these two representative frameworks also have high response latency as shown in Table 2.

**Effect of Number of Retrieved Failure Trial** In experiential learning, we allow the agent to retrieve from failure history with top- $k$  task-relevant trials for reflection generation. To further analyze the potential impact of the number of reflections on action generation, we vary the number of retrieved task-relevant trials  $k$ . As shown in Figure 5, we observe a sharp decrease in both Ele. Acc and Step. SR score as  $k$  increases from 1 to 3. This is because the tasks in MIND2WEB dataset are not highly correlated with each other. Retrieving too many failure experiences would lead to redundant and irrelevant knowledge that distract decision-making.

#### 4.5 Case Study

To intuitively present the advantages of different components, including the dual-process planning mechanism and experiential learning mechanism, we conduct the case study. The example in Figure 6 illustrates the output of keypoints extractor, path finder, reasoning planner, and empirical planner in dual-process planning mechanism. By identifying all constraint requirements and generating plan based on the logic of web design, dual-process planning mechanism effectively enhances the comprehension of complex user instructions and refines the web browsing habits of web agent. Additionally, Figure 7 demonstrates that the experiential learning mechanism can generate reflection from failure history to avoid repeating errors and induce

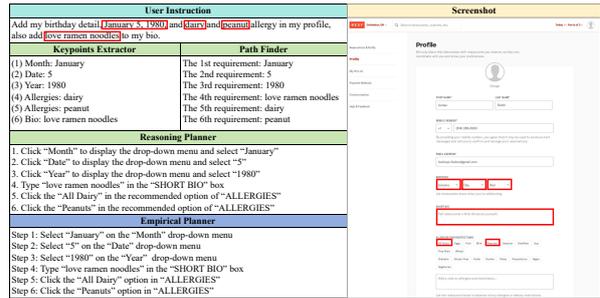

Figure 6: Case study about the dual-process planning.

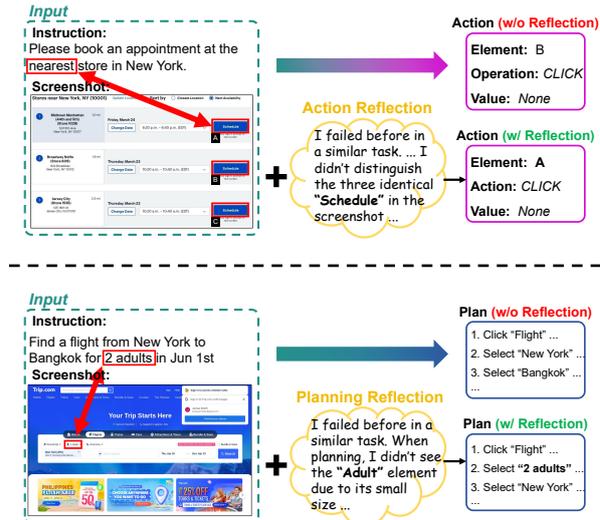

Figure 7: Case study regarding the experiential learning.

better planning and decision-making. Specifically, we present more detailed analysis about these cases in Appendix D.

## 5 Conclusions

In this paper, we propose a multimodal web agent framework called WebExperT, which combines experiential learning with human thought pattern of "thinking fast and slow" to effectively complete automating web navigation like humans. Specifically, we first mark and encode the most important interactive web elements on screenshots. Subsequently, we introduce a dual-process planning mechanism to decompose complex user instructions with fast-and-slow thinking. When failure occurs, the experience will be stored in memory and employed to generate natural language insights through self-reflection, helping agent learn from prior mistakes to continuously optimize its behavior. Our experiments on MIND2WEB benchmark demonstrate that WebExperT outperforms existing methods and achieves new state-of-the-art performance.

## Acknowledgements

This research was supported by the Key-Area Research and Development Program of Guangdong Province (No. 2024B1111100001) and Singapore Ministry of Education (MOE) Academic Research Fund (AcRF) Tier 1 grant (No. MSS24C004).

## Limitations

**Operation Types** There are various types of interactions with websites in real-world web browsing, and we acknowledge the limitation that we haven't supported all possible operations in our framework, including scaling operation and tab-related operations. Scaling operation enables web agents to better identify tiny elements in web screenshots, while tab-related operations provide a more authentic replication of human web browsing habits compared to maintaining everything in a single tab. Consequently, these limitations highlight the need for further research to extend WebExperT with additional operation types to enhance its applicability to real-world websites.

**Element Grounding** As mentioned in Section 4.3, dropping HTML leads to a more significant performance decline compared to dropping screenshot. One of the primary reasons is that our element grounding strategy may result in the overlapping of bounding boxes in screenshot. When numerous elements are densely packed in a screenshot, their bounding boxes and associated labels often overlap together. Such situation often leads to small-sized icons and labels being obscured, significantly hindering the agent's ability to observe and interpret the elements. Actually, these limitations are not exclusive to our work. Existing studies heavily rely on overlaying bounding box to ground the interactive elements in screenshot. Therefore, we acknowledge the need for future research to explore a better element grounding strategy.

**Predefined Criteria** Another limitation of WebExperT is that the strict reliance on predefined failure criteria could reduce the agent's capacity for self-exploration or inhibit creativity. In fact, there are many scenarios where the current step deviates from the groundtruth but the overall task still succeeds. However, this challenge is not unique to our work. Nearly all existing studies employ off-line metrics like Step SR to predefine failure criteria for performance evaluation. Due to the inherent complexity of the web's tree structure, it is

challenging to evaluate the situation of "Different roads lead to Rome" in offline datasets. Therefore, we believe that exploring the balance adherence to ground truth with flexibility in allowing alternative approaches will be a valuable and promising future research direction in web navigation task.

**Transferability and Generalization** We acknowledge the limitation that our framework is only evaluated on automated web navigation task utilizing MIND2WEB dataset. Actually, the modules in our framework, including dual-process planning and experiential learning, rely solely on user instructions, previous action sequences, environment images and being independent of web HTML, which makes them highly adaptable to other tasks and domains. Additionally, the fixed pattern of fast-and-slow thinking usage without any dynamic switching may also limits the flexibility of WebExperT framework. Consequently, there remains room for our future research to integrate our framework into other applications, such as robotic process automation or GUI-based software interactions and explore more flexible fast-and-slow thinking strategy.

## Ethics Statement

We emphasize that the human evaluation experiments in this study adhere strictly to ethical guidelines. Human annotators provided informed consent prior to participating in the study, and their privacy and confidentiality were strictly maintained. No personally identifiable information was collected. Annotators were compensated at a fair rate, ensuring alignment with ethical standards and platform-specific wage guidelines. Hence, the human evaluation experiments are ethically harmless to society.

## References

- Jinze Bai, Shuai Bai, Shusheng Yang, Shijie Wang, Sinan Tan, Peng Wang, Junyang Lin, Chang Zhou, and Jingren Zhou. 2023. Qwen-vl: A versatile vision-language model for understanding, localization, text reading, and beyond. *arXiv preprint arXiv:2308.12966*, 1(2):3.
- Zhe Chen, Jiannan Wu, Wenhai Wang, Weijie Su, Guo Chen, Sen Xing, Muyan Zhong, Qinglong Zhang, Xizhou Zhu, Lewei Lu, et al. 2024. Internvl: Scaling up vision foundation models and aligning for generic visual-linguistic tasks. In *Proceedings of the IEEE/CVF Conference on Computer Vision and Pattern Recognition*, pages 24185–24198.

- Hyung Won Chung, Le Hou, Shayne Longpre, Barret Zoph, Yi Tay, William Fedus, Yunxuan Li, Xuezhi Wang, Mostafa Dehghani, Siddhartha Brahma, Albert Webson, Shixiang Shane Gu, Zhuyun Dai, Mirac Suzgun, Xinyun Chen, Aakanksha Chowdhery, Alex Castro-Ros, Marie Pellat, Kevin Robinson, Dasha Valter, Sharan Narang, Gaurav Mishra, Adams Yu, Vincent Y. Zhao, Yanping Huang, Andrew M. Dai, Hongkun Yu, Slav Petrov, Ed H. Chi, Jeff Dean, Jacob Devlin, Adam Roberts, Denny Zhou, Quoc V. Le, and Jason Wei. 2024. [Scaling instruction-finetuned language models](#). *J. Mach. Learn. Res.*, 25:70:1–70:53.
- Gautier Dagan, Frank Keller, and Alex Lascarides. 2023. [Dynamic planning with a LLM](#). *CoRR*, abs/2308.06391.
- Wenliang Dai, Junnan Li, Dongxu Li, Anthony Meng Huat Tiong, Junqi Zhao, Weisheng Wang, Boyang Li, Pascale Fung, and Steven C. H. Hoi. 2023. [Instructblip: Towards general-purpose vision-language models with instruction tuning](#). In *Advances in Neural Information Processing Systems 36: Annual Conference on Neural Information Processing Systems 2023, NeurIPS 2023, New Orleans, LA, USA, December 10 - 16, 2023*.
- Xiang Deng, Yu Gu, Boyuan Zheng, Shijie Chen, Samuel Stevens, Boshi Wang, Huan Sun, and Yu Su. 2023. [Mind2web: Towards a generalist agent for the web](#). In *Advances in Neural Information Processing Systems 36: Annual Conference on Neural Information Processing Systems 2023, NeurIPS 2023, New Orleans, LA, USA, December 10 - 16, 2023*.
- Yang Deng, An Zhang, Yankai Lin, Xu Chen, Ji-Rong Wen, and Tat-Seng Chua. 2024a. [Large language model powered agents in the web](#). In *Companion Proceedings of the ACM on Web Conference 2024, WWW 2024*, pages 1242–1245. ACM.
- Yang Deng, Xuan Zhang, Wenxuan Zhang, Yifei Yuan, See-Kiong Ng, and Tat-Seng Chua. 2024b. [On the multi-turn instruction following for conversational web agents](#). In *Proceedings of the 62nd Annual Meeting of the Association for Computational Linguistics (Volume 1: Long Papers), ACL 2024, Bangkok, Thailand, August 11-16, 2024*, pages 8795–8812. Association for Computational Linguistics.
- Tim Dettmers, Artidoro Pagnoni, Ari Holtzman, and Luke Zettlemoyer. 2023. [Qlora: Efficient finetuning of quantized llms](#). In *Advances in Neural Information Processing Systems 36: Annual Conference on Neural Information Processing Systems 2023, NeurIPS 2023, New Orleans, LA, USA, December 10 - 16, 2023*.
- Kevin A. Fischer. 2023. [Reflective linguistic programming \(RLP\): A stepping stone in socially-aware AGI \(socialagi\)](#). *CoRR*, abs/2305.12647.
- Hiroki Furuta, Kuang-Huei Lee, Ofir Nachum, Yutaka Matsuo, Aleksandra Faust, Shixiang Shane Gu, and Izzeddin Gur. 2024. [Multimodal web navigation with instruction-finetuned foundation models](#). In *The Twelfth International Conference on Learning Representations, ICLR 2024, Vienna, Austria, May 7-11, 2024*. OpenReview.net.
- Lin Guan, Karthik Valmeekam, Sarath Sreedharan, and Subbarao Kambhampati. 2023. [Leveraging pre-trained large language models to construct and utilize world models for model-based task planning](#). In *Advances in Neural Information Processing Systems 36: Annual Conference on Neural Information Processing Systems 2023, NeurIPS 2023, New Orleans, LA, USA, December 10 - 16, 2023*.
- Izzeddin Gur, Hiroki Furuta, Austin V. Huang, Mustafa Safdari, Yutaka Matsuo, Douglas Eck, and Aleksandra Faust. 2024. [A real-world webagent with planning, long context understanding, and program synthesis](#). In *The Twelfth International Conference on Learning Representations, ICLR 2024, Vienna, Austria, May 7-11, 2024*. OpenReview.net.
- Hongliang He, Wenlin Yao, Kaixin Ma, Wenhao Yu, Yong Dai, Hongming Zhang, Zhenzhong Lan, and Dong Yu. 2024. [Webvoyager: Building an end-to-end web agent with large multimodal models](#). In *Proceedings of the 62nd Annual Meeting of the Association for Computational Linguistics (Volume 1: Long Papers), ACL 2024, Bangkok, Thailand, August 11-16, 2024*, pages 6864–6890. Association for Computational Linguistics.
- Pengcheng He, Xiaodong Liu, Jianfeng Gao, and Weizhu Chen. 2021. [Deberta: decoding-enhanced bert with disentangled attention](#). In *9th International Conference on Learning Representations, ICLR 2021, Virtual Event, Austria, May 3-7, 2021*. OpenReview.net.
- Wenyi Hong, Weihang Wang, Qingsong Lv, Jiazheng Xu, Wenmeng Yu, Junhui Ji, Yan Wang, Zihan Wang, Yuxiao Dong, Ming Ding, and Jie Tang. 2024. [Cogagent: A visual language model for GUI agents](#). In *IEEE/CVF Conference on Computer Vision and Pattern Recognition, CVPR 2024, Seattle, WA, USA, June 16-22, 2024*, pages 14281–14290. IEEE.
- Peter Conway Humphreys, David Raposo, Tobias Pohlen, Gregory Thornton, Rachita Chhaparia, Alistair Muldal, Josh Abramson, Petko Georgiev, Adam Santoro, and Timothy P. Lillicrap. 2022. [A data-driven approach for learning to control computers](#). In *International Conference on Machine Learning, ICML 2022, 17-23 July 2022, Baltimore, Maryland, USA*, volume 162 of *Proceedings of Machine Learning Research*, pages 9466–9482. PMLR.
- Daniel Kahneman. 2011. Thinking, fast and slow. *Farar, Straus and Giroux*.
- Geunwoo Kim, Pierre Baldi, and Stephen McAleer. 2023a. [Language models can solve computer tasks](#). In *Advances in Neural Information Processing Systems 36: Annual Conference on Neural Information*

- Processing Systems 2023, NeurIPS 2023, New Orleans, LA, USA, December 10 - 16, 2023.*
- Geunwoo Kim, Pierre Baldi, and Stephen McAleer. 2023b. [Language models can solve computer tasks](#). In *Advances in Neural Information Processing Systems 36: Annual Conference on Neural Information Processing Systems 2023, NeurIPS 2023, New Orleans, LA, USA, December 10 - 16, 2023*.
- Jaekyeom Kim, Dong-Ki Kim, Lajanugen Logeswaran, Sungryull Sohn, and Honglak Lee. 2024. [Auto-intent: Automated intent discovery and self-exploration for large language model web agents](#). In *Findings of the Association for Computational Linguistics: EMNLP 2024, Miami, Florida, USA, November 12-16, 2024*, pages 16531–16541. Association for Computational Linguistics.
- Kenton Lee, Mandar Joshi, Iulia Raluca Turc, Hexiang Hu, Fangyu Liu, Julian Martin Eisenschlos, Urvashi Khandelwal, Peter Shaw, Ming-Wei Chang, and Kristina Toutanova. 2023. [Pix2struct: Screenshot parsing as pretraining for visual language understanding](#). In *International Conference on Machine Learning, ICML 2023, 23-29 July 2023, Honolulu, Hawaii, USA*, volume 202 of *Proceedings of Machine Learning Research*, pages 18893–18912. PMLR.
- Chin-Yew Lin. 2004. Rouge: A package for automatic evaluation of summaries. In *Text summarization branches out*, pages 74–81.
- Jiaju Lin, Haoran Zhao, Aochi Zhang, Yiting Wu, Huqiyue Ping, and Qin Chen. 2023. [Agentsims: An open-source sandbox for large language model evaluation](#). *CoRR*, abs/2308.04026.
- Evan Zheran Liu, Kelvin Guu, Panupong Pasupat, Tianlin Shi, and Percy Liang. 2018. [Reinforcement learning on web interfaces using workflow-guided exploration](#). In *6th International Conference on Learning Representations, ICLR 2018, Vancouver, BC, Canada, April 30 - May 3, 2018, Conference Track Proceedings*. OpenReview.net.
- Haotian Liu, Chunyuan Li, Qingyang Wu, and Yong Jae Lee. 2023. [Visual instruction tuning](#). In *Advances in Neural Information Processing Systems 36: Annual Conference on Neural Information Processing Systems 2023, NeurIPS 2023, New Orleans, LA, USA, December 10 - 16, 2023*.
- Haohao Luo, Yang Deng, Ying Shen, See-Kiong Ng, and Tat-Seng Chua. 2024. [Chain-of-exemplar: Enhancing distractor generation for multimodal educational question generation](#). In *Proceedings of the 62nd Annual Meeting of the Association for Computational Linguistics (Volume 1: Long Papers), ACL 2024, Bangkok, Thailand, August 11-16, 2024*, pages 7978–7993. Association for Computational Linguistics.
- Kaixin Ma, Hongming Zhang, Hongwei Wang, Xioman Pan, and Dong Yu. 2023. [LASER: LLM agent with state-space exploration for web navigation](#). *CoRR*, abs/2309.08172.
- Sahisnu Mazumder and Oriana Riva. 2021. [FLIN: A flexible natural language interface for web navigation](#). In *Proceedings of the 2021 Conference of the North American Chapter of the Association for Computational Linguistics: Human Language Technologies, NAACL-HLT 2021, Online, June 6-11, 2021*, pages 2777–2788. Association for Computational Linguistics.
- OpenAI. 2023. [GPT-4 technical report](#). *CoRR*, abs/2303.08774.
- Kishore Papineni, Salim Roukos, Todd Ward, and Wei-Jing Zhu. 2002. [Bleu: a method for automatic evaluation of machine translation](#). In *Proceedings of the 40th Annual Meeting of the Association for Computational Linguistics, July 6-12, 2002, Philadelphia, PA, USA*, pages 311–318. ACL.
- Joon Sung Park, Joseph C. O’Brien, Carrie Jun Cai, Meredith Ringel Morris, Percy Liang, and Michael S. Bernstein. 2023. [Generative agents: Interactive simulators of human behavior](#). In *Proceedings of the 36th Annual ACM Symposium on User Interface Software and Technology, UIST 2023, San Francisco, CA, USA, 29 October 2023- 1 November 2023*, pages 2:1–2:22. ACM.
- Alec Radford, Jong Wook Kim, Chris Hallacy, Aditya Ramesh, Gabriel Goh, Sandhini Agarwal, Girish Sastry, Amanda Askell, Pamela Mishkin, Jack Clark, Gretchen Krueger, and Ilya Sutskever. 2021. [Learning transferable visual models from natural language supervision](#). In *Proceedings of the 38th International Conference on Machine Learning, ICML 2021, 18-24 July 2021, Virtual Event*, volume 139 of *Proceedings of Machine Learning Research*, pages 8748–8763. PMLR.
- Peter Shaw, Mandar Joshi, James Cohan, Jonathan Berant, Panupong Pasupat, Hexiang Hu, Urvashi Khandelwal, Kenton Lee, and Kristina Toutanova. 2023. [From pixels to UI actions: Learning to follow instructions via graphical user interfaces](#). In *Advances in Neural Information Processing Systems 36: Annual Conference on Neural Information Processing Systems 2023, NeurIPS 2023, New Orleans, LA, USA, December 10 - 16, 2023*.
- Sheng Shen, Liunian Harold Li, Hao Tan, Mohit Bansal, Anna Rohrbach, Kai-Wei Chang, Zhewei Yao, and Kurt Keutzer. 2022. [How much can CLIP benefit vision-and-language tasks?](#) In *The Tenth International Conference on Learning Representations, ICLR 2022, Virtual Event, April 25-29, 2022*. OpenReview.net.
- Yongliang Shen, Kaitao Song, Xu Tan, Dongsheng Li, Weiming Lu, and Yueting Zhuang. 2023. [Hugging-gpt: Solving AI tasks with chatgpt and its friends in hugging face](#). In *Advances in Neural Information Processing Systems 36: Annual Conference on Neural Information Processing Systems 2023, NeurIPS 2023, New Orleans, LA, USA, December 10 - 16, 2023*.

- Noah Shinn, Federico Cassano, Ashwin Gopinath, Karthik Narasimhan, and Shunyu Yao. 2023. [Reflexion: language agents with verbal reinforcement learning](#). In *Advances in Neural Information Processing Systems 36: Annual Conference on Neural Information Processing Systems 2023, NeurIPS 2023, New Orleans, LA, USA, December 10 - 16, 2023*.
- Chan Hee Song, Brian M. Sadler, Jiaman Wu, Wei-Lun Chao, Clayton Washington, and Yu Su. 2023. [Llm-planner: Few-shot grounded planning for embodied agents with large language models](#). In *IEEE/CVF International Conference on Computer Vision, ICCV 2023, Paris, France, October 1-6, 2023*, pages 2986–2997. IEEE.
- Guanzhi Wang, Yuqi Xie, Yunfan Jiang, Ajay Mandlekar, Chaowei Xiao, Yuke Zhu, Linxi Fan, and Anima Anandkumar. 2024a. [Voyager: An open-ended embodied agent with large language models](#). *Trans. Mach. Learn. Res.*, 2024.
- Xingyao Wang, Zihan Wang, Jiateng Liu, Yangyi Chen, Lifan Yuan, Hao Peng, and Heng Ji. 2024b. [MINT: evaluating llms in multi-turn interaction with tools and language feedback](#). In *The Twelfth International Conference on Learning Representations, ICLR 2024, Vienna, Austria, May 7-11, 2024*. OpenReview.net.
- Zora Zhiruo Wang, Jiayuan Mao, Daniel Fried, and Graham Neubig. 2024c. [Agent workflow memory](#). *CoRR*, abs/2409.07429.
- Jason Wei, Xuezhi Wang, Dale Schuurmans, Maarten Bosma, Brian Ichter, Fei Xia, Ed H. Chi, Quoc V. Le, and Denny Zhou. 2022. [Chain-of-thought prompting elicits reasoning in large language models](#). In *Advances in Neural Information Processing Systems 35: Annual Conference on Neural Information Processing Systems 2022, NeurIPS 2022, New Orleans, LA, USA, November 28 - December 9, 2022*.
- Hengjia Xiao and Peng Wang. 2023. [LLM a\\*: Human in the loop large language models enabled a\\* search for robotics](#). *CoRR*, abs/2312.01797.
- Chengxing Xie and Difan Zou. 2024. [A human-like reasoning framework for multi-phases planning task with large language models](#). *CoRR*, abs/2405.18208.
- Shunyu Yao, Howard Chen, John Yang, and Karthik Narasimhan. 2022. [Webshop: Towards scalable real-world web interaction with grounded language agents](#). In *Advances in Neural Information Processing Systems 35: Annual Conference on Neural Information Processing Systems 2022, NeurIPS 2022, New Orleans, LA, USA, November 28 - December 9, 2022*.
- Shunyu Yao, Dian Yu, Jeffrey Zhao, Izhak Shafran, Tom Griffiths, Yuan Cao, and Karthik Narasimhan. 2023a. [Tree of thoughts: Deliberate problem solving with large language models](#). In *Advances in Neural Information Processing Systems 36: Annual Conference on Neural Information Processing Systems 2023, NeurIPS 2023, New Orleans, LA, USA, December 10 - 16, 2023*.
- Shunyu Yao, Jeffrey Zhao, Dian Yu, Nan Du, Izhak Shafran, Karthik R. Narasimhan, and Yuan Cao. 2023b. [React: Synergizing reasoning and acting in language models](#). In *The Eleventh International Conference on Learning Representations, ICLR 2023, Kigali, Rwanda, May 1-5, 2023*. OpenReview.net.
- Xuan Zhang, Yang Deng, Zifeng Ren, See-Kiong Ng, and Tat-Seng Chua. 2024. [Ask-before-plan: Proactive language agents for real-world planning](#). In *Findings of the Association for Computational Linguistics: EMNLP 2024*, pages 10836–10863. Association for Computational Linguistics.
- Andrew Zhao, Daniel Huang, Quentin Xu, Matthieu Lin, Yong-Jin Liu, and Gao Huang. 2024a. [Expel: LLM agents are experiential learners](#). In *Thirty-Eighth AAAI Conference on Artificial Intelligence, AAAI 2024, Thirty-Sixth Conference on Innovative Applications of Artificial Intelligence, IAAI 2024, Fourteenth Symposium on Educational Advances in Artificial Intelligence, EAAI 2014, February 20-27, 2024, Vancouver, Canada*, pages 19632–19642. AAAI Press.
- Yuze Zhao, Jintao Huang, Jinghan Hu, Xingjun Wang, Yunlin Mao, Daoze Zhang, Zeyinzi Jiang, Zhikai Wu, Baole Ai, Ang Wang, Wenmeng Zhou, and Yingda Chen. 2024b. [SWIFT: A scalable lightweight infrastructure for fine-tuning](#). *CoRR*, abs/2408.05517.
- Zirui Zhao, Wee Sun Lee, and David Hsu. 2023. [Large language models as commonsense knowledge for large-scale task planning](#). In *Advances in Neural Information Processing Systems 36: Annual Conference on Neural Information Processing Systems 2023, NeurIPS 2023, New Orleans, LA, USA, December 10 - 16, 2023*.
- Boyuan Zheng, Boyu Gou, Jihyung Kil, Huan Sun, and Yu Su. 2024a. [Gpt-4v\(ision\) is a generalist web agent, if grounded](#). In *Forty-first International Conference on Machine Learning, ICML 2024, Vienna, Austria, July 21-27, 2024*. OpenReview.net.
- Boyuan Zheng, Boyu Gou, Jihyung Kil, Huan Sun, and Yu Su. 2024b. [Gpt-4v\(ision\) is a generalist web agent, if grounded](#). In *Forty-first International Conference on Machine Learning, ICML 2024, Vienna, Austria, July 21-27, 2024*. OpenReview.net.
- Longtao Zheng, Rundong Wang, Xinrun Wang, and Bo An. 2024c. [Synapse: Trajectory-as-exemplar prompting with memory for computer control](#). In *The Twelfth International Conference on Learning Representations, ICLR 2024, Vienna, Austria, May 7-11, 2024*. OpenReview.net.
- Shuyan Zhou, Frank F. Xu, Hao Zhu, Xuhui Zhou, Robert Lo, Abishek Sridhar, Xianyi Cheng, Tianyue Ou, Yonatan Bisk, Daniel Fried, Uri Alon, and Graham Neubig. 2024. [Webarena: A realistic web environment for building autonomous agents](#). In *The Twelfth International Conference on Learning Representations, ICLR 2024, Vienna, Austria, May 7-11, 2024*. OpenReview.net.

Xizhou Zhu, Yuntao Chen, Hao Tian, Chenxin Tao, Weijie Su, Chenyu Yang, Gao Huang, Bin Li, Lewei Lu, Xiaogang Wang, Yu Qiao, Zhaoxiang Zhang, and Jifeng Dai. 2023. *Ghost in the minecraft: Generally capable agents for open-world environments via large language models with text-based knowledge and memory*. *CoRR*, abs/2305.17144.

## A Implementation Details

**HTML Simplification** Following (Deng et al., 2023), we use Sentence-Transformers<sup>1</sup> and fine-tune DeBERTa-v3-base (He et al., 2021) as the backbone. We employ top-26 ranking results as the candidate pool with labels A to Z. During the training, we set the batch size as 32, the learning rate as  $3e^{-5}$ , and trained for 5 epochs.

**Action Generation** For in-context learning, we use the OpenAI API and experiment with *gpt-4o*. we include three demonstration examples for in-context learning. The complete prompt is shown in Table 10. Note that the action executor  $\mathcal{F}_{action}$  in Stage 1 is only used to generate without updating its parameters, which means skip Step 6 in Algo. 1. And all steps in Stage 2 remain unchanged, which means only the empirical planner will be fine-tuned during training, while the action executor will not. For supervised finetuning, as Flan-T5 has been chosen to be the base model in most research work, we also utilize it as our backbone. Specifically, we use three sizes of Flan-T5 (Chung et al., 2024) as the backbone multimodal LLMs, including Flan-T5-Base, Flan-T5-Large, and Flan-T5-XL. We set the max length of both input and output sequence to 2048. Due to insufficient CUDA memory, we utilize Q-LoRA (Detmers et al., 2023) as our finetune strategy and reduce the batch size to 1. Besides, we finetune the model up to only 1 epoch, with a learning rate of  $1e^{-4}$  and a warmup ratio of 0.03. As For the vision encoder, we leverage the ViT-L/14 336px pretrained from CLIP (Radford et al., 2021) with an image resolution of 2,048.

**Dual-Process Planning** For training empirical planner in intuitive thinking process, We employ InternVL2-8B (Chen et al., 2024) as the backbone multimodal LLM and utilize the default finetuning configuration of SWIFT framework (Zhao et al., 2024b).

In deliberate thinking process, the Keypoints Extractors, Path Finder, and Reasoning Planner are

<sup>1</sup><https://www.sbert.net/examples/applications/cross-encoder/README.html>

all driven by GPT-4o API. The prompts of three modules are shown in Table 11.

**Experiential Learning** For experiential learning, we still employ the off-the-shelf GPT-4o API to extract insights from failure history. The prompts of reflection generation are shown in Table 12. For task-relevant trial retrieval, we first encode the failure trial  $m$  into a semantic vector by also using DeBERTa-v3-base (He et al., 2021)

$$\mathcal{V} = \mathcal{F}_{encode}(m), \quad (8)$$

where  $\mathcal{F}_{encode}(\cdot)$  and  $\mathcal{V}$  denote the encoder and vector representations, respectively. All the vectors lie in a latent sample space that contains rich semantics. If two vectors are close in the latent space, they are more likely to share similar information in analogous field. Subsequently, we calculate the cosine similarity of semantic vector between the current instance and each other failure trial, then retrieve the nearest neighbor in the latent space as the most relevant example:

$$\mathcal{I} = \arg \max_{i \in \{1, 2, \dots, T\}} \max \left( \frac{(\mathcal{V}^i)^T \mathcal{V}}{\|\mathcal{V}^i\|_2 \|\mathcal{V}\|_2} \right), \quad (9)$$

where  $\mathcal{I}$  denotes an index of the most relevant trial among all  $T$  failure trials.

## B Ablation Study of GPT-4o Based WebExperT

To further justify the necessity of each component in our framework, we also conduct an ablation study of WebExperT in ICL setting, as shown in Table 7. Despite being driven by the powerful GPT-4o base model, we can see performance decreases when dropping any components, similar to what is observed in the SFT setting. This confirms the necessity and versatility of all sub-modules in both SFT and ICL settings.

## C Further Analysis of Model Size

To further analyze the resource requirements and model size trade-offs of our WebExperT framework, we conduct comparative experiments utilizing Qwen2.5-VL families, including 3B and 7B versions, as alternative base models. As shown in Table 8, Qwen2.5-VL, which benefits from better pre-training, has superior reasoning and multimodal perception abilities compared to Flan-T5 with the same parameter size (3B). Additionally, as the size

| Method                      | Cross-Task  |             |             | Cross-Website |             |             | Cross-Domain |             |             |
|-----------------------------|-------------|-------------|-------------|---------------|-------------|-------------|--------------|-------------|-------------|
|                             | Ele.Acc     | Op. F1      | Step SR     | Ele.Acc       | Op. F1      | Step SR     | Ele.Acc      | Op. F1      | Step SR     |
| WebExpert                   | <b>45.6</b> | <b>67.4</b> | <b>39.2</b> | <b>39.3</b>   | <b>63.5</b> | <b>36.4</b> | <b>42.9</b>  | <b>64.9</b> | <b>37.1</b> |
| - w/o Intuitive Thinking    | 45.5        | 67.4        | 39.1        | 39.2          | 63.5        | 36.2        | 42.9         | 64.8        | 37.0        |
| - w/o Deliberate Thinking   | 44.0        | 67.0        | 38.5        | 35.4          | 61.9        | 32.8        | 39.3         | 62.7        | 35.0        |
| - w/o Dual-Process Planning | 43.1        | 66.8        | 38.2        | 35.0          | 61.7        | 32.6        | 38.8         | 62.6        | 34.9        |
| - w/o Experiential Learning | 44.7        | 67.0        | 38.4        | 37.5          | 62.3        | 32.9        | 40.2         | 63.7        | 35.5        |
| - w/o Screenshot            | 43.3        | 66.9        | 38.6        | 36.1          | 63.0        | 35.7        | 39.5         | 64.5        | 36.1        |
| - w/o HTML                  | 23.2        | 60.5        | 27.0        | 20.7          | 55.3        | 25.3        | 22.5         | 57.0        | 27.4        |

Table 7: Ablation study of WebExpert with GPT-4o .

| Base Model               | Size | Cross-Task |        |         | Cross-Website |        |         | Cross-Domain |        |         |
|--------------------------|------|------------|--------|---------|---------------|--------|---------|--------------|--------|---------|
|                          |      | Ele.Acc    | Op. F1 | Step SR | Ele.Acc       | Op. F1 | Step SR | Ele.Acc      | Op. F1 | Step SR |
| Flan-T5 <sub>Base</sub>  | 250M | 45.2       | 81.5   | 41.1    | 44.9          | 77.0   | 39.4    | 38.3         | 78.1   | 33.9    |
| Flan-T5 <sub>Large</sub> | 780M | 55.0       | 83.1   | 49.9    | 49.1          | 78.2   | 43.7    | 44.8         | 81.0   | 40.4    |
| Flan-T5 <sub>XL</sub>    | 3B   | 60.3       | 84.4   | 54.9    | 53.9          | 79.6   | 49.0    | 48.5         | 81.5   | 44.0    |
| Qwen2.5-VL               | 3B   | 62.8       | 86.6   | 56.5    | 56.1          | 82.3   | 51.3    | 52.1         | 84.0   | 46.2    |
| Qwen2.5-VL               | 7B   | 71.4       | 93.0   | 63.8    | 65.1          | 91.4   | 57.7    | 61.5         | 92.9   | 55.7    |

Table 8: Detailed performance of our WebExpert framework with different sizes of base models.

of base model increases (250M to 7B), the performance of WebExpert also improves, demonstrating its adaptability to not only low-resource scenarios but also advanced multimodal LLMs. However, we ultimately chose the relatively classical Flan-T5 as the base model because it is commonly used in most existing fine-tuning-based methods, ensuring fairness by avoiding discrepancies arising from differences in the capabilities of base models.

## D Further Analysis of Case Study

### D.1 Dual-Process Planning

We notice that most user instructions provided in real-world web navigation datasets like MIND2WEB often involve numerous constrained requirements (e.g., price). For example, as shown in Figure 6, user instruction "Add my birthday detail, January 5, 1980, and dairy and peanut allergy in my profile, also add love ramen noodles to my bio." describes a scenario where an user aims to update profile with a total of 6 requirements like date. Existing methods often struggle to comprehend such complex instruction and often ignore some of the requirements. To address this common limitation, the keypoints extractor is designed to first identify and extract all the constrained requirements "(1) Month: January (2) Date: 5 (3) Year: 1980 (4) Allergies: dairy (5) Allergies: peanut (6) Bio: love ramen noodles" in instruction. Additionally, existing web agents and humans often exhibit different web browsing habits, especially in their

actions order. Therefore, we introduce path finder to generate a rough route of these keywords on the screenshot "The 1st requirement: January; The 2nd requirement: 5, The 3rd requirement: 1980; ..." based on the human browsing habits (from top to bottom, from left to right). The reasoning planner elaborates on the rough path with supplementary information to generate a comprehensive plan "1. Click "Month" to display the drop-down menu and select "January"; 2. Click "Date" to display the drop-down menu and select "5"; 3. Click "Year" to display the drop-down menu and select "1980" ..." by identifying the corresponding element of each key information in the screenshot. After fine-tuning the empirical planner, the generated empirical plan "Step 1: Select "January" on the "Month" drop-down menu; Step 2: Select "5" on the "Date" drop-down menu; Step 3: Select "1980" on the "Year" drop-down menu; ..." basically covers all important information in the golden plan. Consequently, we can see performance, particularly in Step SR score, improve when integrating the dual-process planning into the framework.

### D.2 Experiential Learning

Figure 7 demonstrates that when faced with the task where there are multiple interactive elements in screenshot with similar or even identical descriptions like the three "Schedule" in red boxes, the web agent often fails to identify the correct one. However, when we add the experiential learning mechanism, the reflection "I failed before in a simi-

| Task                                                                                                               | Action            | Reflection                                                                                                                                                                                                                                                                                                                                                                                                                                                                                                                                                                                      |
|--------------------------------------------------------------------------------------------------------------------|-------------------|-------------------------------------------------------------------------------------------------------------------------------------------------------------------------------------------------------------------------------------------------------------------------------------------------------------------------------------------------------------------------------------------------------------------------------------------------------------------------------------------------------------------------------------------------------------------------------------------------|
| Search for used Jaguar XFs with no black exterior color and save the search as Jaguar to get a notification daily. | Type "Jaguar"     | In this attempt, I was unsuccessful. The mistake occurred in selecting the incorrect VALUE, "jaguar", instead of the specific "jaguar xf," which is essential for accurately executing the user's requirement to search for right models. Next time, I will pay closer attention to the details of the user's plan to ensure that I select and input the precise make and model specified, reducing the chance of errors in task completion.                                                                                                                                                    |
| Find the location and operating hours of the nearest CVS pharmacy to zip code 90028.                               | Click "Element K" | In this attempt, I was unsuccessful. I made mistakes in selecting an element that represented a location result, rather than choosing an element related to submitting the search query. I incorrectly chose an initially displayed option rather than verifying the need to complete the search action tied to the entered zip code. Next time, I will focus on identifying the step within the process that requires user interaction to execute a search, especially after entering search criteria, to find the necessary information like operating hours or locations tied to that query. |

Table 9: Case study of reflection quality.

lar task. ... I didn't distinguish the three identical 'Schedule' in the screenshot ..." generated from failure history helps web agent attach more importance on the context difference between the three "Schedule" elements and avoid repeating errors, leading to a satisfactory decision-making "ELEMENT: A ...". Similarly, when an incorrect plan misleads the decision-making, the reflection "I failed before in a similar task. When planning, I didn't see the 'Adult' element due to its small size ..." would correct the planning errors and induce a better planning. Additionally, we present some cases of generated reflections in Table 9. All reflections contain failure reasons "I made mistakes in ..." and guidance "Next time, I will ...", which are clear and interpretable to optimize agent's decision-making. To further quantify and investigate the quality of generated reflections, we conduct a human evaluation to assess the quality of generated reflections. Specifically, we randomly select the reflections of a subset of 90 tasks from the three test splits and employ 3 annotators to evaluate their appropriateness. We utilize 3 metrics, including **Reflection Accuracy**, **Step Success Rate**, and **Action Refinement Rate**. **Reflection Accuracy** evaluates whether the reflections correctly identify the error location and reasons, while **Action Refinement Rate** evaluates whether the reflections make the agent aware of its mistakes, even if the reflections are not entirely correct. As shown in the table, the reflections generated by our Experiential Learning Module achieves an impressive 84.4% accuracy. Additionally, even when the reflections were not completely correct, the 91.1% Action Refinement Rate demonstrates

that the reflections effectively made the agent aware of its errors. Consequently, we can see performance improvement when integrating the well-designed experiential learning module into the framework.

## E Guideline of Golden Plan Evaluation

We present the guideline of human evaluation for golden plan generated in deliberate thinking process in Figure 8.

| Role      | Content                                                                                                                                                                                                                                                                                                                                                                                                                                                                                                                                                                                                                                                                                                                                                                                                                                                                                                                                                                                                                                                                                                                                                                                                                                                                                                                                                                                                                                                                                                                                                                                                                                                                                                                                                                                 |
|-----------|-----------------------------------------------------------------------------------------------------------------------------------------------------------------------------------------------------------------------------------------------------------------------------------------------------------------------------------------------------------------------------------------------------------------------------------------------------------------------------------------------------------------------------------------------------------------------------------------------------------------------------------------------------------------------------------------------------------------------------------------------------------------------------------------------------------------------------------------------------------------------------------------------------------------------------------------------------------------------------------------------------------------------------------------------------------------------------------------------------------------------------------------------------------------------------------------------------------------------------------------------------------------------------------------------------------------------------------------------------------------------------------------------------------------------------------------------------------------------------------------------------------------------------------------------------------------------------------------------------------------------------------------------------------------------------------------------------------------------------------------------------------------------------------------|
| System    | Imagine that you are imitating humans doing web navigation for a task step by step. At each stage, you can see the webpage like humans by a screenshot and know the previous actions before the current step decided by yourself through recorded history. You need to decide on the first following action to take. You can click on an element with the mouse, select an option, type text or press Enter with the keyboard. (For your understanding, they are like the click(), select_option() and type() functions in playwright respectively) One next step means one operation within the three.                                                                                                                                                                                                                                                                                                                                                                                                                                                                                                                                                                                                                                                                                                                                                                                                                                                                                                                                                                                                                                                                                                                                                                                 |
| User      | <p>Plan: {empirical plan}<br/> Previous Actions: {previous actions}<br/> Task: {task}</p> <p>Combined with the screenshot and each step of the previous action history and their intention and based on the plan, in conjunction with human web browsing habits and the logic of web design, what should be the next action to complete the task? Please select from the following choices:<br/> A: {candidates DOM element A}<br/> B: {candidates DOM element B}<br/> ...<br/> Z: None of the above</p> <p>Conclude your answer using the format below. Ensure your answer is strictly adhering to the format provided below. Please do not leave any explanation in your answers of the final standardized format part, and this final part should be clear and certain. The element choice, action, and value should be in three separate lines.</p> <p>ELEMENT: The uppercase letter of your choice. (No need for PRESS ENTER)<br/> ACTION: Choose an action from {CLICK, SELECT, TYPE, PRESS ENTER, TERMINATE, NONE}.<br/> VALUE: Provide additional input based on ACTION.</p> <p>The VALUE means:<br/> If ACTION == TYPE, specify the text to be typed.<br/> If ACTION == SELECT, indicate the option to be chosen. Revise the selection value to align with the available options within the element.<br/> If ACTION == CLICK, PRESS ENTER, TERMINATE or NONE, write "None".</p> <p>NOTE THAT your answer should strictly contains only 1 ELEMENT, 1 ACTION, and 1 VALUE!!!</p> <p>By the way, you have attempted to solve a similar task before but failed. The following reflection(s) may help you avoid failing the task in the same way you did previously. Use them to improve your strategy of solving the task successfully.<br/> {failure trial}<br/> {reflection}</p> |
| Assistant | <p>ELEMENT: {selected interactive element}<br/> ACTION: {corresponding action}<br/> VALUE: {additional value}</p>                                                                                                                                                                                                                                                                                                                                                                                                                                                                                                                                                                                                                                                                                                                                                                                                                                                                                                                                                                                                                                                                                                                                                                                                                                                                                                                                                                                                                                                                                                                                                                                                                                                                       |

Table 10: Prompt for action generation in WebExperT with GPT models.

| <b>Role</b>               | <b>Content</b>                                                                                                                                                                                                                                                                                                                                                                                                                                                                                                                                                                                                                                                       |
|---------------------------|----------------------------------------------------------------------------------------------------------------------------------------------------------------------------------------------------------------------------------------------------------------------------------------------------------------------------------------------------------------------------------------------------------------------------------------------------------------------------------------------------------------------------------------------------------------------------------------------------------------------------------------------------------------------|
| <b>Keypoint Extractor</b> |                                                                                                                                                                                                                                                                                                                                                                                                                                                                                                                                                                                                                                                                      |
| System                    | Imagine that you are a keypoint extractor. Given a user request and web screenshot, you have to extract all the requirement keypoints like location, date, etc.                                                                                                                                                                                                                                                                                                                                                                                                                                                                                                      |
| User                      | Given the following web navigation task and screenshot, extract the keypoint requirements. Common keypoints consist of location, date, zip, time, amount, price and other important named entity. You can use Named Entity Recognition to assist you in extracting keypoints.<br>Task: {task}<br>Refer to the following examples and imitate their extracting strategy to guide your extraction. Separate the extracted keywords using (1), (2), and (3).<br>Examples:<br>{Example 1}<br>{Example 2}<br>{Example 3}                                                                                                                                                  |
| Assistant                 | Keypoints:<br>(1) {keypoint 1}; (2) {keypoint 2}; ...                                                                                                                                                                                                                                                                                                                                                                                                                                                                                                                                                                                                                |
| <b>Path Finder</b>        |                                                                                                                                                                                                                                                                                                                                                                                                                                                                                                                                                                                                                                                                      |
| System                    | You are a proficient outline generator. Based on the provided keypoints and web screenshot, please give me a rough route for my web navigation plan.                                                                                                                                                                                                                                                                                                                                                                                                                                                                                                                 |
| User                      | Please help me generate a route of my web navigation plan. Try to sort the keypoints to generate a rough route based on human web browsing habits and the logic of web design. Don't include any specific details like action, explanation, thought process, etc. You should use 'The First', 'The Second', 'The Third', etc., to indicate the order of the keypoints. NOTE that In your route, only the keypoints mentioned in input can appear; absolutely no other names are allowed.<br>Keypoints: {keypoints}<br>Refer to the following examples and imitate their strategy to guide your generation.<br>Examples:<br>{Example 1}<br>{Example 2}<br>{Example 3} |
| Assistant                 | Route:<br>(1) The 1st requirement: ...;<br>(2) The 2nd requirement: ...;<br>...                                                                                                                                                                                                                                                                                                                                                                                                                                                                                                                                                                                      |
| <b>Reasoning Planner</b>  |                                                                                                                                                                                                                                                                                                                                                                                                                                                                                                                                                                                                                                                                      |
| System                    | You are a proficient planner. Based on the provided route and web screenshot, please give me a plan for the web navigation task, including specific action and element(e.g. Type the zip code 123456).                                                                                                                                                                                                                                                                                                                                                                                                                                                               |
| User                      | Given the route and web screenshot, you need to generate a plan based on the order of the requirements in route and their corresponding context in web screenshot. Note that all the elements in your plan should be strictly derived from the route. You must strictly adhere to the following format given in the example using (1). (2). (3). as separator. Don't include any specific detailed steps like [span]!<br>Route: {route}<br>Refer to the following examples and imitate their strategy to guide your planning.<br>Examples:<br>{Example 1}<br>{Example 2}<br>{Example 3}                                                                              |
| Assistant                 | Plan:<br>(1) {1st step};<br>(2) {2nd step};<br>...                                                                                                                                                                                                                                                                                                                                                                                                                                                                                                                                                                                                                   |

Table 11: Prompts for three modules in deliberate thinking with GPT models.

| <b>Role</b> | <b>Content</b>                                                                                                                                                                                                                                                                                                                                                                                                                                                                                                                                                                                                                                                                                             |
|-------------|------------------------------------------------------------------------------------------------------------------------------------------------------------------------------------------------------------------------------------------------------------------------------------------------------------------------------------------------------------------------------------------------------------------------------------------------------------------------------------------------------------------------------------------------------------------------------------------------------------------------------------------------------------------------------------------------------------|
| System      | You are an advanced reasoning agent who specializes in analyzing web navigation. You will be presented with a task, an action trajectory, a plan, and your predicted action. Your objective is to provide a concise and clear rationale that explains why the assistant's response made a mistake and how to avoid failing the task in the same way.                                                                                                                                                                                                                                                                                                                                                       |
| User        | Plan: {empirical plan}<br>Previous Actions: {previous actions}<br>Task: {task}<br>Your decision: {action}<br>You have made a wrong decision! The correct action is {groundtruth action}.<br>Compared with the correct action, reflect on your mistakes in the decision-making process, and generate your insights on what will you do when facing a similar task again to avoid failing the task in the same way.<br>Conclude your response using the format below. Ensure your response is strictly adhering to the format provided below.<br>Format:<br>In this attempt, I was unsuccessful. {Where did you make mistakes?}. Next time, I will {your solution to avoid failing the task in the same way} |
| Assistant   | In this attempt, I was unsuccessful. I ignored the floating calender ...                                                                                                                                                                                                                                                                                                                                                                                                                                                                                                                                                                                                                                   |

Table 12: Prompt for reflection generation in WebExperT with GPT models.

| <b>Guideline of Plan Quality Evaluation</b>                                                                                                                                                                                                                                                                                                                                                                                                                                                                                                                                               |                                                                                                                                                                                                                                                                                                                                                                                                                                                                   |
|-------------------------------------------------------------------------------------------------------------------------------------------------------------------------------------------------------------------------------------------------------------------------------------------------------------------------------------------------------------------------------------------------------------------------------------------------------------------------------------------------------------------------------------------------------------------------------------------|-------------------------------------------------------------------------------------------------------------------------------------------------------------------------------------------------------------------------------------------------------------------------------------------------------------------------------------------------------------------------------------------------------------------------------------------------------------------|
| <p>This study aims to evaluate the quality of the web navigation plan. Each case provides you with a task, a list of keypoints, a rough route, and a corresponding website screenshot. You need to evaluate the plans from the following aspects.</p>                                                                                                                                                                                                                                                                                                                                     |                                                                                                                                                                                                                                                                                                                                                                                                                                                                   |
| <b>Case</b>                                                                                                                                                                                                                                                                                                                                                                                                                                                                                                                                                                               |                                                                                                                                                                                                                                                                                                                                                                                                                                                                   |
| <p><b>Task:</b><br/>Find a flight from <b>New York</b> to <b>Bangkok</b> for <b>2 adults</b> in <b>Jun 1st</b>.</p> <p><b>Keypoints:</b><br/>(1) New York; (2) Bangkok; (3) 2 adults; (4) Jun 1st</p> <p><b>Route:</b><br/>2 adults → New York → Bangkok → Jun 1st</p> <p><b>Plan:</b><br/>1. Click “Adult” to display the drop-down menu and select “2”.<br/>2. Type “New York” in the “Departure City or airport” box.<br/>3. Type “Bangkok” in the “Terminal City or airport” box.<br/>4. Click “Departure date” to display the calendar and select the Month “June” and date “1”.</p> | <p><b>Screenshot:</b></p> 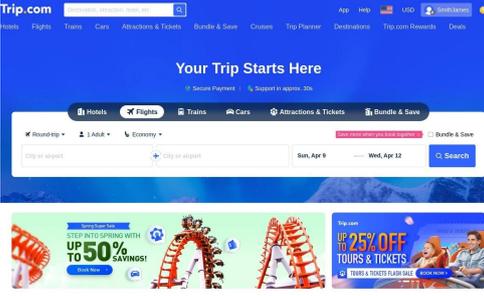                                                                                                                                                                                                                                                                                                                                                      |
| <b>Evaluation</b>                                                                                                                                                                                                                                                                                                                                                                                                                                                                                                                                                                         |                                                                                                                                                                                                                                                                                                                                                                                                                                                                   |
| <p>➤ <b>Relevance:</b> whether the plans capture all the key requirements in user instruction.</p>                                                                                                                                                                                                                                                                                                                                                                                                                                                                                        |                                                                                                                                                                                                                                                                                                                                                                                                                                                                   |
| Options                                                                                                                                                                                                                                                                                                                                                                                                                                                                                                                                                                                   | 1. Completely relevant 2. Quite relevant 3. Moderate relevant<br>4. Mostly irrelevant 5. Completely irrelevant                                                                                                                                                                                                                                                                                                                                                    |
| Examples                                                                                                                                                                                                                                                                                                                                                                                                                                                                                                                                                                                  | 1) “1. Click ‘adult’... 2. Type ‘New York’... 3. Type ‘Bangkok’... 4. Click ‘June’... ‘1’” capture all the keypoints in task exhibits a high level of relevance.<br>2) “1. Type ‘New York’... 2. Type ‘Bangkok’...” demonstrates moderate relevance since it has left out some keypoints such as “2 adults” and “Jun 1st”.<br>3) “1. Click ‘Round-Trip’... 2. Click ‘Economy’” misses all the keypoints in task and even contains completely irrelevant elements. |
| <p>➤ <b>Coherence:</b> whether the orders of plans are aligned with human web browsing habit based on screenshot.</p>                                                                                                                                                                                                                                                                                                                                                                                                                                                                     |                                                                                                                                                                                                                                                                                                                                                                                                                                                                   |
| Options                                                                                                                                                                                                                                                                                                                                                                                                                                                                                                                                                                                   | 1. Completely coherent 2. Mostly coherent 3. Fairly coherent<br>4. Mostly incoherent 5. Completely incoherent                                                                                                                                                                                                                                                                                                                                                     |
| Examples                                                                                                                                                                                                                                                                                                                                                                                                                                                                                                                                                                                  | Humans are used to browsing website from top to bottom, left to right on screenshot.<br>1) “1. Click ‘adult’... 2. Type ‘Bangkok’... 3. Type ‘New York’... 4. Click ‘June’... ‘1’” shows fairly coherent since two of the keypoints are in the wrong order.<br>2) “1. Type ‘Bangkok’... 2. Type ‘New York’... 3. Click ‘June’... ‘1’ 4. Click ‘adult’” is completely incoherent because all the keypoints are in wrong order.                                     |
| <p>➤ <b>Match:</b> whether the operations in plans match the corresponding element in screenshot.</p>                                                                                                                                                                                                                                                                                                                                                                                                                                                                                     |                                                                                                                                                                                                                                                                                                                                                                                                                                                                   |
| Options                                                                                                                                                                                                                                                                                                                                                                                                                                                                                                                                                                                   | 1. Completely matching 2. Quite matching 3. Fairly matching<br>4. Minor matching 5. No matching                                                                                                                                                                                                                                                                                                                                                                   |
| Examples                                                                                                                                                                                                                                                                                                                                                                                                                                                                                                                                                                                  | 1) “1. Click ‘adult’... 2. Type ‘New York’... 3. Type ‘Bangkok’... 4. Type ‘01/06/2024’” is quite matching since it only mistakes the operation of departure date.<br>2) “1. Type ‘adult’... 2. Select ‘New York’... 3. Select ‘Bangkok’... 4. Type ‘01/06/2024’” can’t match any elements in the screenshot at all.                                                                                                                                              |
| <p>➤ <b>Overall:</b> whether the plan is appropriate enough to be the groundtruth overall.</p>                                                                                                                                                                                                                                                                                                                                                                                                                                                                                            |                                                                                                                                                                                                                                                                                                                                                                                                                                                                   |
| Options                                                                                                                                                                                                                                                                                                                                                                                                                                                                                                                                                                                   | 1. Completely appropriate 2. Quite appropriate 3. Moderate appropriate<br>4. Mostly inappropriate 5. Completely inappropriate                                                                                                                                                                                                                                                                                                                                     |
| Examples                                                                                                                                                                                                                                                                                                                                                                                                                                                                                                                                                                                  | “1. Click ‘adult’... 2. Type ‘New York’... 3. Type ‘Bangkok’... 4. Click ‘June’... ‘1’” demonstrates high level of relevance, coherence and totally matches the corresponding element in screenshot. As a whole, the plan is completely suitable to be the groundtruth.                                                                                                                                                                                           |

Figure 8: Guideline of human evaluation for golden plan generation quality.
